# Supplementary material for: Improving Semantic Segmentation in Transformers using Hierarchical Inter-Level Attention
Source: arXiv:2207.02126 source file (2022-07-05)
Supplement: Supplementary file 1 [file appendixE.tex]

% \clearpage
% \section{More Hierarchical Attention Results}
